# Supplementary material for: Generalized dynamical density functional theory for classical fluids and the significance of inertia and hydrodynamic interactions
Source: arXiv:1202.3270 source file (2012-08-08)
Supplement: Supplementary file 1 [file SupplementalMaterial.pdf]

# Supplemental Material

### Derivation of the DDFT

As in the main text, we multiply equation (2) by $\mathbf{p}_1$ and integrate over all but $\mathbf{r}_1$ (denoted $\mathrm{d}\mathbf{r}'$) and obtain an equation for the time evolution of the current $\rho(\mathbf{r}_1,t)\mathbf{v}(\mathbf{r}_1,t) = N/m \int \mathrm{d}\mathbf{p}\mathrm{d}\mathbf{r}'\mathbf{p}_1 f^{(N)}(\mathbf{r},\mathbf{p},t)$:

$$
\begin{aligned}
0 = {} & \partial_t\big(\rho(\mathbf{r}_1,t)\mathbf{v}(\mathbf{r}_1,t)\big) + \gamma\rho(\mathbf{r}_1,t)\mathbf{v}(\mathbf{r}_1,t) \\
& + \frac{N}{m}\int \mathrm{d}\mathbf{r}'\boldsymbol{\nabla}_{\mathbf{r}_1} V(\mathbf{r},t)\rho^{(N)}(\mathbf{r},t) && \text{(V)} \\
& + \frac{N\gamma}{m}\sum_{j=1}^{N}\int \mathrm{d}\mathbf{p}\mathrm{d}\mathbf{r}'\tilde{\boldsymbol{\Gamma}}_{1j}(\mathbf{r})\mathbf{p}_j f^{(N)}(\mathbf{r},\mathbf{p},t) && \text{(H)} \\
& + \boldsymbol{\nabla}_{\mathbf{r}_1}\cdot\int \mathrm{d}\mathbf{p}_1 \frac{\mathbf{p}_1\otimes\mathbf{p}_1}{m^2} f^{(1)}(\mathbf{r}_1,\mathbf{p}_1,t). && \text{(K)}
\end{aligned}
$$

Here $f^{(1)}(\mathbf{r}_1,\mathbf{p}_1,t) = N\int \mathrm{d}\mathbf{p}'\mathrm{d}\mathbf{r}' f^{(N)}(\mathbf{r},\mathbf{p},t)$ is the one-body phase-space distribution and $\rho^{(N)}(\mathbf{r},t) = \int \mathrm{d}\mathbf{p} f^{(N)}(\mathbf{r},\mathbf{p},t)$ is the $N$-body position distribution. Further, we have written $\boldsymbol{\Gamma}(\mathbf{r}) = \gamma[\mathbf{1} + \tilde{\boldsymbol{\Gamma}}(\mathbf{r})]$, where the HI tensor $\tilde{\boldsymbol{\Gamma}}$ is decomposed into $3\times 3$ blocks $\tilde{\boldsymbol{\Gamma}}_{ij}$ [11]. Here $\mathbf{1}$ is the $3N\times 3N$ identity matrix and $\gamma$ is the friction felt by a single, isolated particle. Physically, $\tilde{\boldsymbol{\Gamma}}_{ij}$ describes how the momentum of particle $j$ generates a force on particle $i$. At this point our derivation is still rigorous, but to close this equation as a functional of $\rho$ and $\mathbf{v}$, it is necessary to deal with terms arising from the many-body part of the potential in (V), HI in (H), and 'kinetic pressure' effects in (K). This is achieved, as detailed in the main text, via the adiabatic approximation (V), the choice of $g$ in $f^{(2)}(\mathbf{r}_1,\mathbf{r}_2,\mathbf{p}_1,\mathbf{p}_2,t) = f^{(1)}(\mathbf{r}_1,\mathbf{p}_1,t)f^{(1)}(\mathbf{r}_1,\mathbf{p}_1,t)g(\mathbf{r}_1,\mathbf{r}_2,[\rho])$ (H) and the local equilibrium approximation (K).

### Friction and diffusion tensors

Since $\boldsymbol{\Gamma}$ in (1) must be positive-definite, we use the inverse of the Rotne-Prager approximation with hydrodynamic diameter $\sigma_{\mathrm{H}} = 0.5$ [8]. This choice of $\sigma_{\mathrm{H}}$ justifies both neglecting lubrication forces and using a two-body expansion. For the DDFT (3) and (4) we use the 11-term two-body expansion given by Jeffrey and Onishi [24]. Whilst not strictly equivalent, the two descriptions are similar when the particles are well-separated in terms of the hydrodynamic diameter. In the overdamped limit, the Rotne-Prager approximation to the diffusion tensor is used for both stochastic and DDFT calculations.

### Correlation functional

An extension to our choice of $g$ would be to use the analytic correlation function based on the Percus-Yevick equation [31]. However, the volume-exclusion approximation suffices for the systems studied here, as demonstrated by the very good agreement between the DDFT and stochastic simulations.


[31] A. Trokhymchuk, I. Nezbeda, J. Jirsák, and D. Henderson. Hard-sphere radial distribution function again. *J. Chem. Phys.* **123** 024501 (2005).


# Supplemental Movie Legends

### Supplemental Movie 1

Motion of nine identical hard-sphere colloidal particles, coloured by initial symmetry, under a constant vertical force and HI at zero temperature (solution of (1) ).
*(right movie)* Dynamics, from left to right starting from a symmetric initial condition, for a slightly perturbed initial condition, and (in black) without hydrodynamic interactions. Camera follows the centre of mass frame of the particles without hydrodynamic interactions. Note, in particular, the increased velocity due to HI.
*(left movie)* Magnified view in the centre of mass frame of the particles with HI.

### Supplemental Movie 2

A representative stochastic realization of the dynamics of 50 particles with diameter one and friction coefficient $\gamma = 6$. The initial distribution is chosen from the equilibrium distribution in potential $V$ with $r_0 = 5$,

which is instantaneously switched to $r_0 = 0$ at time zero. Note the noisy, Brownian-motion-like, behaviour of the particles. Colour denotes radial position, *purple* denoting less than 2, *green* otherwise.

**Supplemental Movie 3**

Radial particle distribution and velocity given by *(smooth curves)* solution of DDFT (3) and (4) versus *(noisy curves)* stochastic equations (1) with *(blue)* and without *(red)* HI. Also shown are the mean radial positions and velocities. The system contains 50 particles, with $\gamma = 6$, and starts at equilibrium in potential $V$ with $r_0 = 5$, which is instantaneously switched to $r_0 = 0$ at time zero. Note, in particular, that HI have a damping effect on the dynamics.

**Supplemental Movie 4**

Radial particle distribution and velocity given by solution of DDFT (3) and (4) with *(blue)* and without *(red)* HI. Also shown are the mean radial positions and velocities. The system contains 500 particles, with $\gamma = 10$, and starts at equilibrium in potential $V$ with $r_0 = 5$, which is instantaneously switched to $r_0 = 0$ at time zero. Note, in particular, the quantitative differences introduced by the inclusion of HI.

## Supplemental Figure

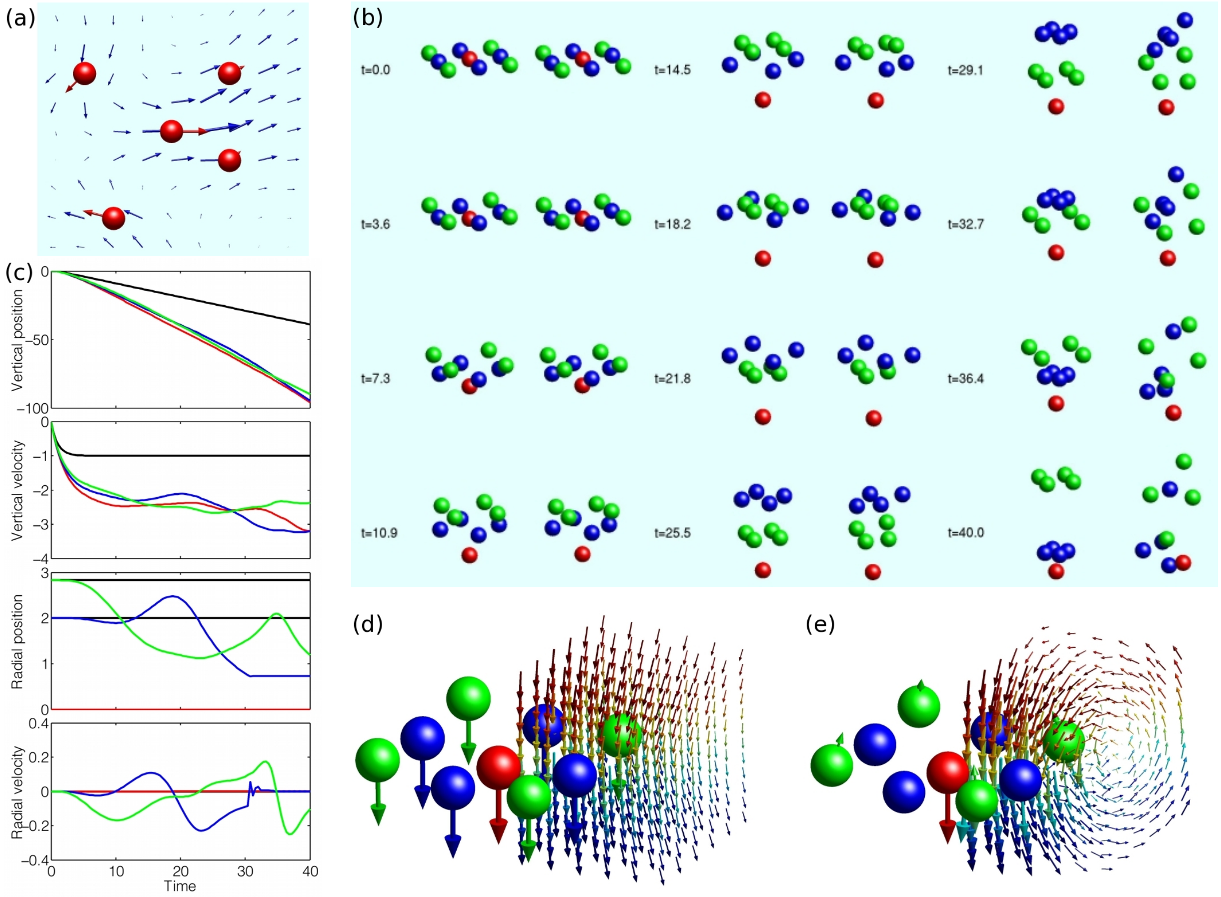


Figure 4: Dynamics of hydrodynamically-interacting particles. (a) Bath fluid flows *(blue)* induced by motion of spherical colloidal particles *(red)* restricted to a plane. (b)–(e): Motion of nine identical hard-sphere colloidal particles, coloured by symmetry, under a constant vertical force and HI at zero temperature (solution of (1)). (b) Evolution in the centre of mass frames with *(left)* completely symmetric square lattice and *(right)* slightly perturbed initial conditions. (c) Vertical and radial (from centre particle in horizontal plane) positions and velocities of corresponding coloured particles for symmetric initial condition. Black curves correspond to no HI. The kink in the blue radial velocity curve is due to the omission of lubrication forces. Colloid velocities and bath flows in (d) laboratory reference frame and (e) centre of mass frame. Bath flow coloured by vertical position. Other quadrants are symmetric. See also Supplemental Movie 1.
